# Supplementary material for: Cohesion and excitations of diamond-structure silicon by quantum Monte Carlo: Benchmarks and control of systematic biases
Source: arXiv:2102.11998 ancillary file (2021-05-21)
Supplement: Supplementary file 1 [file Diamond_Si_Supp.pdf]

# **Supplemental Material for “Cohesion and excitations in diamond Si by quantum Monte Carlo methods: benchmarks and systematic biases”**

Abdulgani Annaberdiyev<sup>1</sup>, Guangming Wang<sup>1</sup>, Cody A. Melton<sup>2</sup>, M. Chandler Bennett<sup>3</sup>, Lubos Mitas<sup>1</sup>

*1) Department of Physics, North Carolina State University, Raleigh, North Carolina 27695-8202, USA*

*2) Sandia National Laboratories, Albuquerque, New Mexico 87123, USA and*

*3) Materials Science and Technology Division, Oak Ridge National Laboratory, Oak Ridge, Tennessee, 37831, USA*

## I. GEOMETRY

TABLE 1: Direct lattice vectors Cartesian components. Primitive cell. (Angstrom)

| X    | Y    | Z    |
|------|------|------|
| 2.71 | 2.71 | 0.00 |
| 0.00 | 2.71 | 2.71 |
| 2.71 | 0.00 | 2.71 |

TABLE 2: Atomic positions in the primitive cell. Cartesian coordinates. (Angstrom)

| X       | Y       | Z       |
|---------|---------|---------|
| 0.6775  | 0.6775  | 0.6775  |
| -0.6775 | -0.6775 | -0.6775 |

## II. ATOMIC ENERGIES

TABLE 3: Atomic energies [Ha] used in this work. Employed aug-cc-pVnZ basis sets are shown for each method.

| State | Method        | Energy [Ha]   |
|-------|---------------|---------------|
| GS    | FCI (TZ-6Z)   | -3.762073(57) |
| GS    | DMC/HF        | -3.7601(1)    |
| GS    | ROHF (6Z)     | -3.67247779   |
| GS    | UCCSD(T) (6Z) | -3.76088094   |
| CA    | ROHF (6Z)     | -3.39077973   |
| CA    | UCCSD(T) (6Z) | -3.46103571   |
| AN    | ROHF (6Z)     | -3.70823500   |
| AN    | UCCSD(T) (6Z) | -3.81279591   |

### III. TOTAL ENERGIES

TABLE 4: QMCPACK/PBE total energies [Ha] at  $k = \Gamma$  for  $n = [8, 64, 216]$  atoms. Calculations for Slater WFN without Jastrow (S) and Slater-Jastrow WFN (SJ) are shown. DMC timestep is  $0.0025 \text{ Ha}^{-1}$ .  $n$  is the number of atoms. AN( $\Gamma$ /X) represents an extra electron added to the conduction  $k = \Gamma$ /X point.

| State          | Method | WFN | $n = 8$      | $n = 64$      | $n = 216$     |
|----------------|--------|-----|--------------|---------------|---------------|
| GS             | VMC    | S   | -30.2354(6)  | -242.2753(27) | -817.0897(23) |
| GS             | VMC    | SJ  | -31.1587(5)  | -251.1578(13) | -848.1912(12) |
| GS             | DMC    | SJ  | -31.2457(9)  | -251.5702(22) | -849.2468(35) |
| $\Gamma\Gamma$ | VMC    | S   | -30.1028(5)  | -242.0868(25) | -816.8788(27) |
| $\Gamma\Gamma$ | VMC    | SJ  | -31.0439(4)  | -251.0227(10) | -848.0547(16) |
| $\Gamma\Gamma$ | DMC    | SJ  | -31.1344(10) | -251.4338(25) | -849.1081(31) |
| $\Gamma X$     | VMC    | S   | -30.1857(4)  | -242.1817(22) | -816.9651(17) |
| $\Gamma X$     | VMC    | SJ  | -31.1242(4)  | -251.1077(7)  | -848.1366(8)  |
| $\Gamma X$     | DMC    | SJ  | -31.2149(10) | -251.5164(19) | -849.1945(45) |
| CA             | VMC    | S   | -30.4965(4)  | -242.5156(27) | -817.3213(19) |
| CA             | VMC    | SJ  | -31.3905(3)  | -251.3755(4)  | -848.4080(9)  |
| CA             | DMC    | SJ  | -31.4771(9)  | -251.7891(22) | -849.4721(30) |
| AN( $\Gamma$ ) | VMC    | S   | -29.8442(3)  | -241.8537(24) | -816.6532(17) |
| AN( $\Gamma$ ) | VMC    | SJ  | -30.8153(3)  | -250.8053(5)  | -847.8367(8)  |
| AN( $\Gamma$ ) | DMC    | SJ  | -30.9056(9)  | -251.2213(24) | -848.9063(37) |
| AN(X)          | VMC    | S   | -29.9305(3)  | -241.9467(23) | -816.7409(20) |
| AN(X)          | VMC    | SJ  | -30.8992(3)  | -250.8896(8)  | -847.9204(8)  |
| AN(X)          | DMC    | SJ  | -30.9917(9)  | -251.3005(23) | -848.9833(38) |

TABLE 5: QMCPACK/PBE0 total energies [Ha] at  $k = \Gamma$  for  $n = [8, 64, 216]$  atoms. Notations are as in Table 4.

| State          | Method | WFN | $n = 8$     | $n = 64$      | $n = 216$     |
|----------------|--------|-----|-------------|---------------|---------------|
| GS             | VMC    | S   | -30.2478(5) | -242.4541(18) | -817.8381(14) |
| GS             | VMC    | SJ  | -31.1609(8) | -251.1697(4)  | -848.2195(5)  |
| GS             | DMC    | SJ  | -31.2440(9) | -251.5744(13) | -849.2688(30) |
| $\Gamma\Gamma$ | VMC    | S   | -30.1155(4) | -242.2576(10) | -817.6114(13) |
| $\Gamma\Gamma$ | VMC    | SJ  | -31.0458(2) | -251.0358(3)  | -848.0805(7)  |
| $\Gamma\Gamma$ | DMC    | SJ  | -31.1360(4) | -251.4371(10) | -849.1225(25) |
| $\Gamma X$     | VMC    | S   | -30.2036(4) | -242.3498(9)  | -817.7056(18) |
| $\Gamma X$     | VMC    | SJ  | -31.1315(8) | -251.1190(7)  | -848.1652(6)  |
| $\Gamma X$     | DMC    | SJ  | -31.2214(9) | -251.5198(13) | -849.2123(25) |

TABLE 6: QMCPACK/HF total energies [Ha] at  $k = \Gamma$  for  $n = [8, 64, 216]$  atoms. Notations are as in Table 4.

| State          | Method | WFN | $n = 8$      | $n = 64$      | $n = 216$     |
|----------------|--------|-----|--------------|---------------|---------------|
| GS             | VMC    | S   | -30.2664(6)  | -242.7106(26) | -818.8121(20) |
| GS             | VMC    | SJ  | -31.1479(4)  | -250.9287(7)  | -847.2472(8)  |
| GS             | DMC    | SJ  | -31.2370(9)  | -251.4369(18) | -848.7195(44) |
| $\Gamma\Gamma$ | VMC    | S   | -30.1246(5)  | -242.4981(19) | -818.5652(22) |
| $\Gamma\Gamma$ | VMC    | SJ  | -31.0284(2)  | -250.7860(7)  | -847.0966(7)  |
| $\Gamma\Gamma$ | DMC    | SJ  | -31.1233(10) | -251.2869(16) | -848.5496(30) |
| CA             | VMC    | S   | -30.5234(4)  | -242.9370(18) |               |
| CA             | VMC    | SJ  | -31.3792(2)  | -251.1467(4)  |               |
| CA             | DMC    | SJ  | -31.4712(8)  | -251.6466(22) |               |
| AN( $\Gamma$ ) | VMC    | S   | -29.8748(4)  | -242.2783(19) |               |
| AN( $\Gamma$ ) | VMC    | SJ  | -30.8026(4)  | -250.5701(6)  |               |
| AN( $\Gamma$ ) | DMC    | SJ  | -30.8971(7)  | -251.0770(25) |               |

TABLE 7: QWalk/HF total energies [Ha] at  $k = \Gamma$  for  $n = [8, 64, 216]$  atoms. Notations are as in Table 4.

| State          | Method | WFN | $n = 8$     | $n = 64$      | $n = 216$     |
|----------------|--------|-----|-------------|---------------|---------------|
| GS             | VMC    | S   | -30.2028(2) | -242.2588(24) | -817.3037(49) |
| GS             | VMC    | SJ  | -31.0912(2) | -250.5267(25) |               |
| GS             | DMC    | SJ  | -31.2132(6) | -251.2646(38) |               |
| $\Gamma\Gamma$ | VMC    | S   | -30.0707(2) | -242.0586(29) | -817.0550(66) |
| $\Gamma\Gamma$ | VMC    | SJ  | -30.9776(1) | -250.3750(12) |               |
| $\Gamma\Gamma$ | DMC    | SJ  | -31.1027(4) | -251.1099(19) |               |

## IV. KINETIC ENERGIES

TABLE 8: QMCPACK/PBE kinetic energies [Ha] at  $k = \Gamma$  for  $n = [8, 64, 216]$  atoms. Notations are as in Table 4.

| State          | Method | WFN | $n = 8$      | $n = 64$     | $n = 216$    |
|----------------|--------|-----|--------------|--------------|--------------|
| GS             | VMC    | S   | 13.44518(69) | 101.0104(26) | 338.2343(35) |
| GS             | VMC    | SJ  | 14.0448(15)  | 107.2227(71) | 360.546(10)  |
| GS             | DMC    | SJ  | 14.0332(47)  | 107.184(32)  | 360.124(40)  |
| $\Gamma\Gamma$ | VMC    | S   | 13.41978(41) | 100.9890(40) | 338.2148(30) |
| $\Gamma\Gamma$ | VMC    | SJ  | 14.0395(13)  | 107.1961(96) | 360.512(10)  |
| $\Gamma\Gamma$ | DMC    | SJ  | 14.0156(47)  | 107.164(21)  | 360.055(89)  |
| $\Gamma X$     | VMC    | S   | 13.23495(38) | 100.7970(33) | 338.0289(23) |
| $\Gamma X$     | VMC    | SJ  | 13.8615(12)  | 107.0150(28) | 360.3395(44) |
| $\Gamma X$     | DMC    | SJ  | 13.8423(46)  | 106.970(10)  | 360.116(19)  |
| CA             | VMC    | S   | 12.77672(57) | 100.3425(28) | 337.5707(35) |
| CA             | VMC    | SJ  | 13.3830(12)  | 106.5371(21) | 359.8638(44) |
| CA             | DMC    | SJ  | 13.3791(34)  | 106.555(11)  | 359.661(24)  |
| AN( $\Gamma$ ) | VMC    | S   | 14.08869(30) | 101.6585(32) | 338.8809(25) |
| AN( $\Gamma$ ) | VMC    | SJ  | 14.6960(16)  | 107.8666(36) | 361.2058(45) |
| AN( $\Gamma$ ) | DMC    | SJ  | 14.6715(52)  | 107.816(17)  | 360.950(52)  |
| AN(X)          | VMC    | S   | 13.90362(29) | 101.4678(29) | 338.6991(31) |
| AN(X)          | VMC    | SJ  | 14.52369(95) | 107.6897(40) | 361.0224(45) |
| AN(X)          | DMC    | SJ  | 14.4909(46)  | 107.6655(85) | 360.789(22)  |

TABLE 9: QMCPACK/PBE0 kinetic energies [Ha] at  $k = \Gamma$  for  $n = [8, 64, 216]$  atoms. Notations are as in Table 4.

| State          | Method | WFN | $n = 8$     | $n = 64$     | $n = 216$    |
|----------------|--------|-----|-------------|--------------|--------------|
| GS             | VMC    | S   | 13.3866(6)  | 100.8091(24) | 337.9964(17) |
| GS             | VMC    | SJ  | 14.0442(33) | 107.3619(24) | 361.2548(34) |
| GS             | DMC    | SJ  | 14.0348(56) | 107.3469(98) | 361.039(34)  |
| $\Gamma\Gamma$ | VMC    | S   | 13.3594(6)  | 100.7851(13) | 337.9678(18) |
| $\Gamma\Gamma$ | VMC    | SJ  | 14.0289(10) | 107.3880(12) | 361.2317(57) |
| $\Gamma\Gamma$ | DMC    | SJ  | 14.0158(15) | 107.341(12)  | 360.948(38)  |
| $\Gamma X$     | VMC    | S   | 13.1700(6)  | 100.5959(11) | 337.7787(17) |
| $\Gamma X$     | VMC    | SJ  | 13.8532(24) | 107.1537(26) | 361.0409(48) |
| $\Gamma X$     | DMC    | SJ  | 13.8484(48) | 107.1475(86) | 360.788(21)  |

TABLE 10: QMCPACK/HF kinetic energies [Ha] at  $k = \Gamma$  for  $n = [8, 64, 216]$  atoms. Notations are as in Table 4.

| State          | Method | WFN | $n = 8$      | $n = 64$     | $n = 216$    |
|----------------|--------|-----|--------------|--------------|--------------|
| GS             | VMC    | S   | 13.45750(68) | 102.3825(29) | 344.3498(28) |
| GS             | VMC    | SJ  | 14.1348(14)  | 108.7970(44) | 366.1020(59) |
| GS             | DMC    | SJ  | 14.0946(40)  | 108.358(11)  | 364.712(17)  |
| $\Gamma\Gamma$ | VMC    | S   | 13.41877(59) | 102.3443(30) | 344.3097(23) |
| $\Gamma\Gamma$ | VMC    | SJ  | 14.10483(49) | 108.7505(39) | 366.0644(58) |
| $\Gamma\Gamma$ | DMC    | SJ  | 14.0656(41)  | 108.3454(99) | 364.669(40)  |
| CA             | VMC    | S   | 12.79356(46) | 101.7230(25) |              |
| CA             | VMC    | SJ  | 13.46995(64) | 108.1202(19) |              |
| CA             | DMC    | SJ  | 13.4501(40)  | 107.686(16)  |              |
| AN( $\Gamma$ ) | VMC    | S   | 14.08181(53) | 103.0108(24) |              |
| AN( $\Gamma$ ) | VMC    | SJ  | 14.7702(19)  | 109.4274(27) |              |
| AN( $\Gamma$ ) | DMC    | SJ  | 14.7264(39)  | 109.008(21)  |              |

# V. TOTAL ENERGIES PER ATOM

TABLE 11: QMCPACK/PBE energies per atom [Ha] at  $k = \Gamma$  for  $n = [8, 64, 216]$  atoms and for thermodynamic limit (TDL) using  $n = 64, 216$  atom extrapolations. Calculations for Slater WFN without Jastrow (S) and Slater-Jastrow WFN (SJ) are shown. DMC timestep is  $0.0025 \text{ Ha}^{-1}$ .  $n$  is the number of atoms. AN( $\Gamma$ /X) represents an extra electron added to the conduction  $k = \Gamma$ /X point.

| State          | Method | WFN | $n = 8$     | $n = 64$     | $n = 216$    | TDL          |
|----------------|--------|-----|-------------|--------------|--------------|--------------|
| GS             | VMC    | S   | -3.77942(7) | -3.78555(4)  | -3.78282(1)  | -3.78167(2)  |
| GS             | VMC    | SJ  | -3.89484(6) | -3.92434(2)  | -3.926811(6) | -3.92785(1)  |
| GS             | DMC    | SJ  | -3.9057(1)  | -3.93078(3)  | -3.93170(2)  | -3.93208(3)  |
| $\Gamma\Gamma$ | VMC    | S   | -3.76285(6) | -3.78261(4)  | -3.78185(1)  | -3.78153(2)  |
| $\Gamma\Gamma$ | VMC    | SJ  | -3.88049(5) | -3.92223(2)  | -3.926179(7) | -3.92784(1)  |
| $\Gamma\Gamma$ | DMC    | SJ  | -3.8918(1)  | -3.92865(4)  | -3.93106(1)  | -3.93207(3)  |
| $\Gamma X$     | VMC    | S   | -3.77321(5) | -3.78409(3)  | -3.782246(8) | -3.78147(2)  |
| $\Gamma X$     | VMC    | SJ  | -3.89052(5) | -3.92356(1)  | -3.926558(4) | -3.927822(7) |
| $\Gamma X$     | DMC    | SJ  | -3.9019(1)  | -3.92994(3)  | -3.93146(2)  | -3.93209(3)  |
| CA             | VMC    | S   | -3.81206(5) | -3.78931(4)  | -3.783895(9) | -3.78162(2)  |
| CA             | VMC    | SJ  | -3.92381(4) | -3.927742(6) | -3.927815(4) | -3.927845(6) |
| CA             | DMC    | SJ  | -3.9346(1)  | -3.93420(3)  | -3.93274(1)  | -3.93213(2)  |
| AN( $\Gamma$ ) | VMC    | S   | -3.73053(4) | -3.77896(4)  | -3.780802(8) | -3.78158(2)  |
| AN( $\Gamma$ ) | VMC    | SJ  | -3.85191(4) | -3.918833(8) | -3.925170(4) | -3.927838(6) |
| AN( $\Gamma$ ) | DMC    | SJ  | -3.8632(1)  | -3.92533(4)  | -3.93012(2)  | -3.93214(3)  |
| AN(X)          | VMC    | S   | -3.74131(4) | -3.78042(4)  | -3.781208(9) | -3.78154(2)  |
| AN(X)          | VMC    | SJ  | -3.86240(4) | -3.92015(1)  | -3.925557(4) | -3.927834(7) |
| AN(X)          | DMC    | SJ  | -3.8740(1)  | -3.92657(4)  | -3.93048(2)  | -3.93212(3)  |

TABLE 12: QMCPACK/PBE0 energies per atom [Ha] at  $k = \Gamma$  for  $n = [8, 64, 216]$  atoms and for thermodynamic limit (TDL) using  $n = 64, 216$  atom extrapolations. Notations are as in Table 11.

| State          | Method | WFN | $n = 8$     | $n = 64$     | $n = 216$    | TDL          |
|----------------|--------|-----|-------------|--------------|--------------|--------------|
| GS             | VMC    | S   | -3.78098(6) | -3.78835(3)  | -3.786288(6) | -3.78542(2)  |
| GS             | VMC    | SJ  | -3.8951(1)  | -3.924527(6) | -3.926942(2) | -3.927959(4) |
| GS             | DMC    | SJ  | -3.9055(1)  | -3.93085(2)  | -3.93180(1)  | -3.93220(2)  |
| $\Gamma\Gamma$ | VMC    | S   | -3.76444(5) | -3.78527(2)  | -3.785238(6) | -3.78522(1)  |
| $\Gamma\Gamma$ | VMC    | SJ  | -3.88072(3) | -3.922434(5) | -3.926299(3) | -3.927926(5) |
| $\Gamma\Gamma$ | DMC    | SJ  | -3.89200(5) | -3.92870(2)  | -3.93112(1)  | -3.93214(2)  |
| $\Gamma X$     | VMC    | S   | -3.77545(5) | -3.78672(1)  | -3.785674(8) | -3.78524(1)  |
| $\Gamma X$     | VMC    | SJ  | -3.8914(1)  | -3.92373(1)  | -3.926691(3) | -3.927936(6) |
| $\Gamma X$     | DMC    | SJ  | -3.9027(1)  | -3.93000(2)  | -3.93154(1)  | -3.93219(2)  |

TABLE 13: QMCPACK/HF energies per atom [Ha] at  $k = \Gamma$  for  $n = [8, 64, 216]$  atoms and for thermodynamic limit (TDL) using  $n = 64, 216$  atom extrapolations. Notations are as in Table 11.

| State          | Method | WFN | $n = 8$     | $n = 64$     | $n = 216$    | TDL          |
|----------------|--------|-----|-------------|--------------|--------------|--------------|
| GS             | VMC    | S   | -3.78330(7) | -3.79235(4)  | -3.790797(9) | -3.79014(2)  |
| GS             | VMC    | SJ  | -3.89349(5) | -3.92076(1)  | -3.922441(4) | -3.923148(7) |
| GS             | DMC    | SJ  | -3.9046(1)  | -3.92870(3)  | -3.92926(2)  | -3.92949(3)  |
| $\Gamma\Gamma$ | VMC    | S   | -3.76558(6) | -3.78903(3)  | -3.78965(1)  | -3.78992(2)  |
| $\Gamma\Gamma$ | VMC    | SJ  | -3.87855(3) | -3.91853(1)  | -3.921744(3) | -3.923096(7) |
| $\Gamma\Gamma$ | DMC    | SJ  | -3.8904(1)  | -3.92636(3)  | -3.92847(1)  | -3.92936(2)  |
| CA             | VMC    | S   | -3.81542(5) | -3.79589(3)  |              |              |
| CA             | VMC    | SJ  | -3.92240(3) | -3.924167(6) |              |              |
| CA             | DMC    | SJ  | -3.9339(1)  | -3.93198(3)  |              |              |
| AN( $\Gamma$ ) | VMC    | S   | -3.73435(5) | -3.78560(3)  |              |              |
| AN( $\Gamma$ ) | VMC    | SJ  | -3.85033(5) | -3.915158(9) |              |              |
| AN( $\Gamma$ ) | DMC    | SJ  | -3.86214(9) | -3.92308(4)  |              |              |

TABLE 14: QWalk/HF energies per atom [Ha] at  $k = \Gamma$  for  $n = [8, 64, 216]$  atoms and for thermodynamic limit (TDL) using  $n = 64, 216$  atom extrapolations. Notations are as in Table 11.

| State          | Method | WFN | $n = 8$     | $n = 64$    | $n = 216$   | TDL         |
|----------------|--------|-----|-------------|-------------|-------------|-------------|
| GS             | VMC    | S   | -3.77535(3) | -3.78529(4) | -3.78381(2) | -3.78319(4) |
| GS             | VMC    | SJ  | -3.88640(3) | -3.91448(4) |             |             |
| GS             | DMC    | SJ  | -3.90165(7) | -3.92601(6) |             |             |
| $\Gamma\Gamma$ | VMC    | S   | -3.75884(3) | -3.78217(5) | -3.78266(3) | -3.78287(5) |
| $\Gamma\Gamma$ | VMC    | SJ  | -3.87220(1) | -3.91211(2) |             |             |
| $\Gamma\Gamma$ | DMC    | SJ  | -3.88784(5) | -3.92359(3) |             |             |

# VI. KINETIC ENERGIES PER ATOM

TABLE 15: QMCPACK/PBE kinetic energies per atom [Ha] at  $k = \Gamma$  for  $n = [8, 64, 216]$  atoms and for thermodynamic limit (TDL) using  $n = 64, 216$  atom extrapolations. Notations are as in Table 11.

| State          | Method | WFN | $n = 8$    | $n = 64$   | $n = 216$  | TDL        |
|----------------|--------|-----|------------|------------|------------|------------|
| GS             | VMC    | S   | 1.68065(9) | 1.57829(4) | 1.56590(2) | 1.56068(3) |
| GS             | VMC    | SJ  | 1.7556(2)  | 1.6754(1)  | 1.66919(5) | 1.66660(8) |
| GS             | DMC    | SJ  | 1.7542(6)  | 1.6747(5)  | 1.6672(2)  | 1.6641(3)  |
| $\Gamma\Gamma$ | VMC    | S   | 1.67747(5) | 1.57795(6) | 1.56581(1) | 1.56070(3) |
| $\Gamma\Gamma$ | VMC    | SJ  | 1.7549(2)  | 1.6749(1)  | 1.66904(5) | 1.66655(9) |
| $\Gamma\Gamma$ | DMC    | SJ  | 1.7519(6)  | 1.6744(3)  | 1.6669(4)  | 1.6638(6)  |
| $\Gamma X$     | VMC    | S   | 1.65437(5) | 1.57495(5) | 1.56495(1) | 1.56074(3) |
| $\Gamma X$     | VMC    | SJ  | 1.7327(1)  | 1.67211(4) | 1.66824(2) | 1.66661(3) |
| $\Gamma X$     | DMC    | SJ  | 1.7303(6)  | 1.6714(2)  | 1.66720(9) | 1.6654(1)  |
| CA             | VMC    | S   | 1.59709(7) | 1.56785(4) | 1.56283(2) | 1.56071(3) |
| CA             | VMC    | SJ  | 1.6729(1)  | 1.66464(3) | 1.66604(2) | 1.66662(3) |
| CA             | DMC    | SJ  | 1.6724(4)  | 1.6649(2)  | 1.6651(1)  | 1.6652(2)  |
| AN( $\Gamma$ ) | VMC    | S   | 1.76109(4) | 1.58841(5) | 1.56889(1) | 1.56067(3) |
| AN( $\Gamma$ ) | VMC    | SJ  | 1.8370(2)  | 1.68542(6) | 1.67225(2) | 1.66671(4) |
| AN( $\Gamma$ ) | DMC    | SJ  | 1.8339(6)  | 1.6846(3)  | 1.6711(2)  | 1.6654(4)  |
| AN(X)          | VMC    | S   | 1.73795(4) | 1.58543(5) | 1.56805(1) | 1.56073(3) |
| AN(X)          | VMC    | SJ  | 1.8155(1)  | 1.68265(6) | 1.67140(2) | 1.66666(4) |
| AN(X)          | DMC    | SJ  | 1.8114(6)  | 1.6823(1)  | 1.6703(1)  | 1.6653(2)  |

TABLE 16: QMCPACK/PBE0 kinetic energies per atom [Ha] at  $k = \Gamma$  for  $n = [8, 64, 216]$  atoms and for thermodynamic limit (TDL) using  $n = 64, 216$  atom extrapolations. Quantum Espresso PBE0 kinetic energy per atom: 1.56221466 Ha. Notations are as in Table 11.

| State          | Method | WFN | $n = 8$    | $n = 64$   | $n = 216$   | TDL        |
|----------------|--------|-----|------------|------------|-------------|------------|
| GS             | VMC    | S   | 1.67332(7) | 1.57514(4) | 1.564798(8) | 1.56044(2) |
| GS             | VMC    | SJ  | 1.7555(4)  | 1.67753(4) | 1.67248(2)  | 1.67035(3) |
| GS             | DMC    | SJ  | 1.7544(7)  | 1.6773(2)  | 1.6715(2)   | 1.6690(2)  |
| $\Gamma\Gamma$ | VMC    | S   | 1.66993(7) | 1.57477(2) | 1.564666(8) | 1.56041(1) |
| $\Gamma\Gamma$ | VMC    | SJ  | 1.7536(1)  | 1.67794(2) | 1.67237(3)  | 1.67002(4) |
| $\Gamma\Gamma$ | DMC    | SJ  | 1.7520(2)  | 1.6772(2)  | 1.6711(2)   | 1.6685(3)  |
| $\Gamma X$     | VMC    | S   | 1.64625(7) | 1.57181(2) | 1.563790(8) | 1.56041(1) |
| $\Gamma X$     | VMC    | SJ  | 1.7316(3)  | 1.67428(4) | 1.67149(2)  | 1.67031(4) |
| $\Gamma X$     | DMC    | SJ  | 1.7310(6)  | 1.6742(1)  | 1.6703(1)   | 1.6687(1)  |

TABLE 17: QMCPACK/HF kinetic energies per atom [Ha] at  $k = \Gamma$  for  $n = [8, 64, 216]$  atoms and for thermodynamic limit (TDL) using  $n = 64, 216$  atom extrapolations. Notations are as in Table 11.

| State          | Method | WFN | $n = 8$    | $n = 64$   | $n = 216$  | TDL        |
|----------------|--------|-----|------------|------------|------------|------------|
| GS             | VMC    | S   | 1.68219(9) | 1.59973(5) | 1.59421(1) | 1.59189(3) |
| GS             | VMC    | SJ  | 1.7669(2)  | 1.69995(7) | 1.69492(3) | 1.69280(5) |
| GS             | DMC    | SJ  | 1.7618(5)  | 1.6931(2)  | 1.68848(8) | 1.6865(1)  |
| $\Gamma\Gamma$ | VMC    | S   | 1.67735(7) | 1.59913(5) | 1.59403(1) | 1.59188(2) |
| $\Gamma\Gamma$ | VMC    | SJ  | 1.76310(6) | 1.69923(6) | 1.69474(3) | 1.69285(5) |
| $\Gamma\Gamma$ | DMC    | SJ  | 1.7582(5)  | 1.6929(2)  | 1.6883(2)  | 1.6863(3)  |
| CA             | VMC    | S   | 1.59919(6) | 1.58942(4) |            |            |
| CA             | VMC    | SJ  | 1.68374(8) | 1.68938(3) |            |            |
| CA             | DMC    | SJ  | 1.6813(5)  | 1.6826(3)  |            |            |
| AN( $\Gamma$ ) | VMC    | S   | 1.76023(7) | 1.60954(4) |            |            |
| AN( $\Gamma$ ) | VMC    | SJ  | 1.8463(2)  | 1.70980(4) |            |            |
| AN( $\Gamma$ ) | DMC    | SJ  | 1.8408(5)  | 1.7032(3)  |            |            |

## VII. VARIANCE TO ENERGY RATIO

TABLE 18: QMCPACK/PBE variance/(total energy) at  $k = \Gamma$  for  $n = [8, 64, 216]$  atoms. Calculations for Slater WFN without Jastrow (S) and Slater-Jastrow WFN (SJ) are shown. DMC timestep is  $0.0025 \text{ Ha}^{-1}$ .  $n$  is the number of atoms. AN( $\Gamma/X$ ) represents an extra electron added to the conduction  $k = \Gamma/X$  point.

| State          | Method | WFN | $n = 8$    | $n = 64$    | $n = 216$   |
|----------------|--------|-----|------------|-------------|-------------|
| GS             | VMC    | S   | 0.1124(4)  | 0.1174(2)   | 0.11882(8)  |
| GS             | VMC    | SJ  | 0.01255(3) | 0.00737(2)  | 0.006657(9) |
| GS             | DMC    | SJ  | 0.01230(2) | 0.00727(1)  | 0.00660(2)  |
| $\Gamma\Gamma$ | VMC    | S   | 0.1134(4)  | 0.1181(3)   | 0.1192(1)   |
| $\Gamma\Gamma$ | VMC    | SJ  | 0.01307(2) | 0.00743(2)  | 0.00665(1)  |
| $\Gamma\Gamma$ | DMC    | SJ  | 0.01280(2) | 0.00733(1)  | 0.00662(3)  |
| $\Gamma X$     | VMC    | S   | 0.1120(3)  | 0.1176(2)   | 0.1191(1)   |
| $\Gamma X$     | VMC    | SJ  | 0.0129(1)  | 0.007412(8) | 0.00669(2)  |
| $\Gamma X$     | DMC    | SJ  | 0.01246(2) | 0.00730(2)  | 0.00659(1)  |
| CA             | VMC    | S   | 0.1053(3)  | 0.1169(2)   | 0.1188(2)   |
| CA             | VMC    | SJ  | 0.01190(2) | 0.00734(1)  | 0.00667(3)  |
| CA             | DMC    | SJ  | 0.01156(3) | 0.00724(2)  | 0.00657(1)  |
| AN( $\Gamma$ ) | VMC    | S   | 0.1203(2)  | 0.1187(3)   | 0.1192(1)   |
| AN( $\Gamma$ ) | VMC    | SJ  | 0.01355(6) | 0.00750(2)  | 0.006674(4) |
| AN( $\Gamma$ ) | DMC    | SJ  | 0.01319(2) | 0.00738(2)  | 0.00661(1)  |
| AN(X)          | VMC    | S   | 0.1199(5)  | 0.1184(2)   | 0.1193(1)   |
| AN(X)          | VMC    | SJ  | 0.01340(2) | 0.00747(1)  | 0.00671(3)  |
| AN(X)          | DMC    | SJ  | 0.01311(3) | 0.00737(2)  | 0.00661(2)  |

TABLE 19: QMCPACK/PBE0 variance/(total energy) at  $k = \Gamma$  for  $n = [8, 64, 216]$  atoms. Notations are as in Table 18.

| State          | Method | WFN | $n = 8$     | $n = 64$    | $n = 216$   |
|----------------|--------|-----|-------------|-------------|-------------|
| GS             | VMC    | S   | 0.1123(4)   | 0.1173(2)   | 0.11871(8)  |
| GS             | VMC    | SJ  | 0.01255(3)  | 0.00737(2)  | 0.006657(9) |
| GS             | DMC    | SJ  | 0.01230(2)  | 0.00727(1)  | 0.00660(2)  |
| $\Gamma\Gamma$ | VMC    | S   | 0.1133(4)   | 0.1180(3)   | 0.1191(1)   |
| $\Gamma\Gamma$ | VMC    | SJ  | 0.01258(2)  | 0.00727(1)  | 0.00665(1)  |
| $\Gamma\Gamma$ | DMC    | SJ  | 0.012246(6) | 0.007160(5) | 0.00662(3)  |
| $\Gamma X$     | VMC    | S   | 0.1120(3)   | 0.1175(2)   | 0.1190(1)   |
| $\Gamma X$     | VMC    | SJ  | 0.0129(1)   | 0.007411(8) | 0.00669(2)  |
| $\Gamma X$     | DMC    | SJ  | 0.01245(2)  | 0.00730(2)  | 0.00659(1)  |

TABLE 20: QMCPACK/HF variance/(total energy) at  $k = \Gamma$  for  $n = [8, 64, 216]$  atoms. Notations are as in Table 18.

| State          | Method | WFN | $n = 8$    | $n = 64$   | $n = 216$   |
|----------------|--------|-----|------------|------------|-------------|
| GS             | VMC    | S   | 0.1103(4)  | 0.1149(7)  | 0.1150(1)   |
| GS             | VMC    | SJ  | 0.01218(1) | 0.00747(3) | 0.007002(4) |
| GS             | DMC    | SJ  | 0.01206(2) | 0.00741(1) | 0.00702(1)  |
| $\Gamma\Gamma$ | VMC    | S   | 0.1116(6)  | 0.1146(3)  | 0.1152(2)   |
| $\Gamma\Gamma$ | VMC    | SJ  | 0.01261(1) | 0.00750(2) | 0.007033(8) |
| $\Gamma\Gamma$ | DMC    | SJ  | 0.01238(2) | 0.00747(1) | 0.00701(2)  |

### VIII. QMC/HF GAPS

TABLE 21: QMC/HF gaps [eV] using extensive total energies for  $n = [8, 64, 216]$  atoms. Calculations for Slater WFN without Jastrow (S) and Slater-Jastrow WFN (SJ) are shown.

| Gap                       | Method | WFN | $n = 8$ | $n = 64$ | $n = 216$ |
|---------------------------|--------|-----|---------|----------|-----------|
| Promotion gaps $E_g$      |        |     |         |          |           |
| $\Gamma\Gamma$            | VMC    | S   | 3.86(2) | 5.78(9)  | 6.72(8)   |
| $\Gamma\Gamma$            | VMC    | SJ  | 3.25(1) | 3.88(3)  | 4.10(3)   |
| $\Gamma\Gamma$            | DMC    | SJ  | 3.09(4) | 4.08(7)  | 4.6(1)    |
| Quasi-Particle gaps $E_G$ |        |     |         |          |           |
| $\Gamma\Gamma$            | VMC    | S   | 3.66(4) | 5.6(2)   |           |
| $\Gamma\Gamma$            | VMC    | SJ  | 3.10(2) | 3.83(4)  |           |
| $\Gamma\Gamma$            | DMC    | SJ  | 2.88(6) | 4.1(1)   |           |

TABLE 22: QMC/HF gaps [eV] using intensive energies and slopes for free- and constrained- fits. Calculations for Slater WFN without Jastrow (S) and Slater-Jastrow WFN (SJ) are shown.

| Gap                  | Method | WFN | free-fit | const-fit |
|----------------------|--------|-----|----------|-----------|
| Promotion gaps $E_g$ |        |     |          |           |
| $\Gamma\Gamma$       | VMC    | S   | 5.4(1)   | 6.2(5)    |
| $\Gamma\Gamma$       | VMC    | SJ  | 3.79(4)  | 4.0(1)    |
| $\Gamma\Gamma$       | DMC    | SJ  | 3.9(1)   | 4.2(2)    |

## IX. DFT ENERGIES

TABLE 23: Quantum Espresso kinetic energy cutoff convergence for PBE WFN. Primitive cell.  $k : [3 \times 3 \times 3]$ . 100 Ry was used in the paper.

| Ecutoff (Ry) | PBE Energy (Ry) |
|--------------|-----------------|
| 20           | -15.64225520    |
| 40           | -15.65431430    |
| 60           | -15.65550986    |
| 80           | -15.65561567    |
| 100          | -15.65564165    |
| 120          | -15.65565192    |
| 140          | -15.65565801    |
| 160          | -15.65566211    |

TABLE 24: Quantum Espresso  $k$ -mesh convergence. Ecutoff = 100 Ry. Meshes are  $\Gamma$  centered and correspond to the conventional cell.  $k : [6 \times 6 \times 6]$  in the conventional cell was used in the paper.

| $k$ -mesh | PBE Energy (Ry) |
|-----------|-----------------|
| 6x6x6     | -15.70327831    |
| 12x12x12  | -15.70329659    |

TABLE 25: Quantum Espresso convergence of the three-dimensional mesh for  $q$  ( $k_1 - k_2$ ) sampling of the Fock operator. Ecutoff = 100 Ry. Here primitive cell is used with  $[12 \times 12 \times 12]$   $k$ -mesh centered at  $\Gamma$ .  $q : [6 \times 6 \times 6]$  and Ecutoff(fock) = 250 Ry was used in the paper.

| $q$ -mesh | HF Energy (Ry) | $\Gamma\Gamma$ gap (eV) |
|-----------|----------------|-------------------------|
| 1x1x1     | -15.43109152   | 14.8383                 |
| 2x2x2     | -15.19349722   | 11.1389                 |
| 3x3x3     | -15.15852082   | 9.7913                  |
| 4x4x4     | -15.15497694   | 9.3266                  |
| 6x6x6     | -15.15513626   | 9.1047                  |

TABLE 26: Quantum Espresso gaps [eV]. Kinetic energies per atom (KE/ $n$ ) [Ha] are shown as well.

| Method | $\Gamma\Gamma$ [eV] | $\Gamma X$ [eV] | (KE/ $n$ ) [Ha] |
|--------|---------------------|-----------------|-----------------|
| PBE    | 2.565               | 0.623           | 1.56302235      |
| PBE0   | 3.962               | 1.839           | 1.56221466      |
| HF     | 9.107               | 6.572           | 1.59267264      |

TABLE 27: CRYSTAL gaps [eV]. Kinetic energies per atom (KE/ $n$ ) [Ha] are shown as well.

| Method | $\Gamma\Gamma$ [eV] | $\Gamma X$ [eV] | (KE/ $n$ ) [Ha] |
|--------|---------------------|-----------------|-----------------|
| PBE    | 2.5973              | 0.6815          | 1.55596214      |
| PBE0   | 3.9113              | 1.8539          | 1.55527351      |

TABLE 28: CRYSTAL energies [Ha] using TZVP basis set.

| $n$ | Total Energy | Kinetic Energy |
|-----|--------------|----------------|
| 2   | -7.564802    | 3.165914       |
| 8   | -30.259234   | 12.665212      |
| 64  | -242.074418  | 101.30854      |
| 216 | -817.001164  | 341.919338     |

## X. MPC INTERACTION ENERGIES

TABLE 29: QMCPACK/PBE0 total energies [Ha] at  $k = \Gamma$  for  $n = 8$  atoms. Calculations for Slater WFN without Jastrow (S) and Slater-Jastrow WFN (SJ) are shown. DMC timestep is  $0.0025 \text{ Ha}^{-1}$ .  $n$  is the number of atoms. Model Periodic Coloumb (MPC) interaction was used. Proliferation of walkers are also via MPC. Jastrow factors were re-optimized for each state.

| State          | Method | WFN | $n = 8$     |
|----------------|--------|-----|-------------|
| GS             | VMC    | S   | -30.0031(3) |
| GS             | VMC    | SJ  | -31.0003(3) |
| GS             | DMC    | SJ  | -31.1215(4) |
| $\Gamma\Gamma$ | VMC    | S   | -29.8622(4) |
| $\Gamma\Gamma$ | VMC    | SJ  | -30.8832(3) |
| $\Gamma\Gamma$ | DMC    | SJ  | -31.0109(5) |
| $\Gamma X$     | VMC    | S   | -29.9475(3) |
| $\Gamma X$     | VMC    | SJ  | -30.9672(3) |
| $\Gamma X$     | DMC    | SJ  | -31.0942(4) |

TABLE 30: QMCPACK/PBE0 kinetic energies per atom [Ha] at  $k = \Gamma$  for  $n = 8$  atoms. Details are as in Tab. 29.

| State          | Method | WFN | $n = 8$    |
|----------------|--------|-----|------------|
| GS             | VMC    | S   | 1.67334(4) |
| GS             | VMC    | SJ  | 1.7636(1)  |
| GS             | DMC    | SJ  | 1.7605(2)  |
| $\Gamma\Gamma$ | VMC    | S   | 1.66990(5) |
| $\Gamma\Gamma$ | VMC    | SJ  | 1.7623(1)  |
| $\Gamma\Gamma$ | DMC    | SJ  | 1.7591(3)  |
| $\Gamma X$     | VMC    | S   | 1.64639(6) |
| $\Gamma X$     | VMC    | SJ  | 1.7403(1)  |
| $\Gamma X$     | DMC    | SJ  | 1.7373(2)  |

TABLE 31: QMC/PBE0 gaps [eV] using extensive total energies for  $n = 8$  atoms. Details are as in Tab. 29.

| Gap                  | Method | WFN | $n = 8$ |
|----------------------|--------|-----|---------|
| Promotion gaps $E_g$ |        |     |         |
| $\Gamma\Gamma$       | VMC    | S   | 3.83(1) |
| $\Gamma\Gamma$       | VMC    | SJ  | 3.19(1) |
| $\Gamma\Gamma$       | DMC    | SJ  | 3.01(2) |
| $\Gamma X$           | VMC    | S   | 1.51(1) |
| $\Gamma X$           | VMC    | SJ  | 0.90(1) |
| $\Gamma X$           | DMC    | SJ  | 0.74(2) |

## XI. TIME-STEP BIAS

To quantify the time-step bias in this work, we considered the 8 atom cell at various time-steps. Figure 1 shows this study. One can see that the time-step used in this work ( $t = 0.0025 \text{ Ha}^{-1}$ ) is within the error bars of the extrapolated value.

FIG. 1: DMC energies of the 8 atom cell at  $k = \Gamma$  point. The square symbol shows the linearly extrapolated zero-time-step energy.

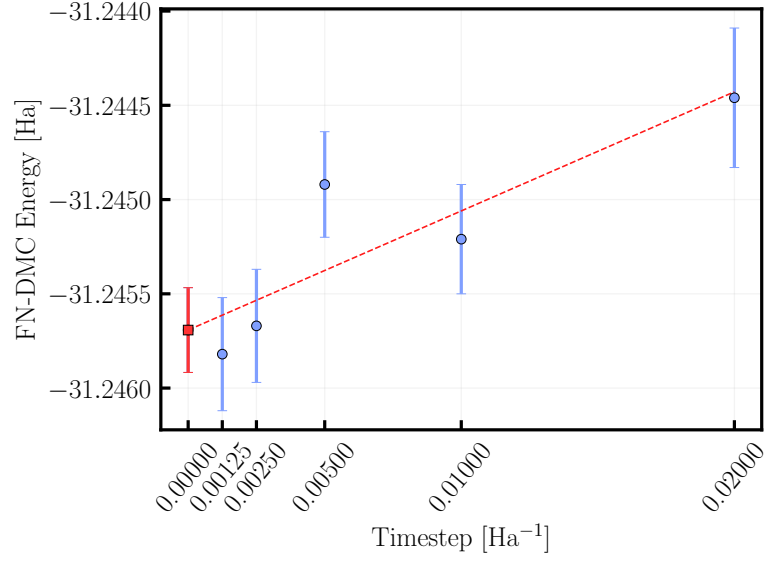

## XII. WALKER POPULATION BIAS

Figure 2 shows the DMC energies versus the number of target walkers. We can see that for this system size (8 atoms),  $\sim 550$  walkers give the same energy within the error bars compared to the largest population tested. Using this data, we estimated the number of walkers required for the larger sizes which would result in walker-population-bias-free energies assuming linear relationship with the system size. This is shown in Table 32. We can see that enough walkers were used for all system sizes. Therefore, we conclude that there is negligible walker population bias within the given errors.

FIG. 2: DMC energies of the 8 atom cell at  $k = \Gamma$  point. DMC timestep of  $0.0025 \text{ Ha}^{-1}$  was used.  $x$ -axis is plotted in  $\log_2$  scale. Dashed lines are guide to the eye.

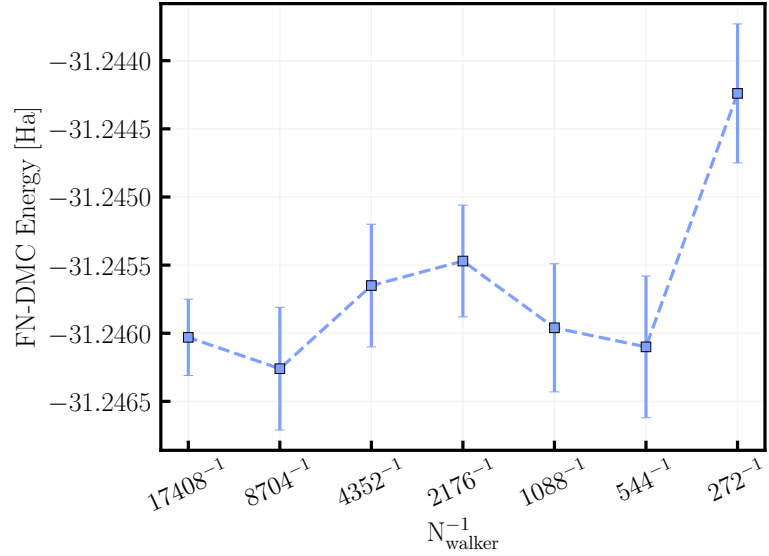

TABLE 32: The estimated walker population for bias-free energies ( $N_{\text{walker}}(\text{bias-free})$ ) and the actual target population used ( $N_{\text{walker}}(\text{used-target})$ ).

| $n$ | $N_{\text{walker}}(\text{bias-free})$ | $N_{\text{walker}}(\text{used-target})$ |
|-----|---------------------------------------|-----------------------------------------|
| 8   | 550                                   | 2048                                    |
| 64  | 4400                                  | 8192                                    |
| 216 | 14850                                 | 16384                                   |

Sandia National Laboratories is a multimission laboratory managed and operated by National Technology & Engineering Solutions of Sandia, LLC, a wholly owned subsidiary of Honeywell International Inc., for the U.S. Department of Energy's National Nuclear Security Administration under contract DE-NA0003525.

This paper describes objective technical results and analysis. Any subjective views or opinions that might be expressed in the paper do not necessarily represent the views of the U.S. Department of Energy or the United States Government.
